# Supplementary material for: Controllable Subspaces in Structured Networks of Hierarchical Directed Acyclic Graphs: Controllability of Individual Nodes
Source: arXiv:2403.01184 ancillary file (2025-01-11)
Supplement: Supplementary file 1 [file Supplementary_Materials.pdf]

# Supplementary Materials for "Controllable Subspaces in Structured Networks of Hierarchical Directed Acyclic Graphs: Controllability of Individual Nodes" in IEEE-TAC

Nam-Jin Park[1], Yeong-Ung Kim[1], Koog-Hwan Oh[2], and Hyo-Sung Ahn[1]

**Abstract**

This article is supplementary material to the technical note titled "Controllable Subspaces in Structured Networks of Hierarchical Directed Acyclic Graphs: Controllability of Individual Nodes," submitted to IEEE Transactions on Automatic Control (TAC) by the same authors. Based on the preliminaries outlined in the technical note, this supplement maintains consistent numbering of Theorems, Propositions, and Lemmas as presented in the note. It offers additional insights, detailed explanations, and examples that complement the concepts discussed in the technical note and is referenced accordingly throughout.

## I. Numerical and Topological Examples

This section provides examples to facilitate understanding of the concepts presented in our technical note. The following example illustrates the difference between structural and strong structural controllability in structured networks.

**Example 1.** *Let us consider a graph $\mathcal{G}(\mathcal{V},\mathcal{E})$ with a leader $1 \in \mathcal{V}_\mathcal{L}$ as shown in Fig. 2(a). Then, the corresponding structured network is characterized by the following $\mathcal{A}_\mathcal{P}$ and $\mathcal{B}$:*

$$\mathcal{A}_\mathcal{P} = \begin{bmatrix} 0 & a_{12} & 0 \\ a_{21} & 0 & a_{23} \\ a_{31} & a_{32} & 0 \end{bmatrix}, \quad \mathcal{B} = \begin{bmatrix} 1 \\ 0 \\ 0 \end{bmatrix}. \tag{1}$$

*The controllability matrix for the pair $(\mathcal{A}_\mathcal{P}, \mathcal{B})$ is given by:*

$$\mathcal{C} = [\mathcal{B}, \mathcal{A}_\mathcal{P}\mathcal{B}] = \begin{bmatrix} 1 & 0 & a_{12}a_{21} \\ 0 & a_{21} & a_{23}a_{31} \\ 0 & a_{31} & a_{21}a_{32} \end{bmatrix}. \tag{2}$$

*The above controllability matrix has full rank if $a_{23}a_{31}^2 \neq a_{21}^2 a_{32}$ holds. However, it reduces to rank 2 for specific realizations of network parameters, e.g., $a_{23}a_{31}^2 = a_{21}^2 a_{32}$. Therefore, while the given structured network in* (1) *is structurally controllable, it is not strongly structurally controllable due to uncontrollable exceptions.*

The following example demonstrates the necessity and significance of the fixed controllable subspace in structured networks from the perspective of state controllability.

**Example 2.** *Let us consider a graph $\mathcal{G}(\mathcal{V},\mathcal{E})$ with a leader $1 \in \mathcal{V}_\mathcal{L}$ as shown in Fig. 2(b). Then, the corresponding structured network is characterized by the following $\mathcal{A}_\mathcal{P}$ and $\mathcal{B}$:*

$$\mathcal{A}_\mathcal{P} = \begin{bmatrix} 0 & a_{12} & 0 \\ 0 & 0 & 0 \\ 0 & a_{32} & 0 \end{bmatrix}, \quad \mathcal{B} = \begin{bmatrix} 0 \\ 1 \\ 0 \end{bmatrix}. \tag{3}$$

*The controllability matrix for the pair $(\mathcal{A}_\mathcal{P}, \mathcal{B})$ is given by:*

$$\mathcal{C} = \begin{bmatrix} 0 & a_{12} & 0 \\ 1 & 0 & 0 \\ 0 & a_{32} & 0 \end{bmatrix}. \tag{4}$$

*Note that the rank of the above controllability matrix is 2 for all network parameters, e.g., $a_{12}$ and $a_{32}$, therefore the Structurally Controllable Subspace (SCS) and Strongly Structurally Controllable Subspace (SSCS) are identical. For simplicity, we will explain this example in terms of SCS. The SCS of the structured network, as defined by* (3)*, reflects the column space of the*

[1]School of Mechanical Engineering, Gwangju Institute of Science and Technology (GIST), Gwangju, Korea. E-mails: namjinpark@gist. ac.kr; yeongungkim@gm.gist.ac.kr; hyosung@gist.ac.kr;
[2]Smart Electrics Research Center, Korea Electronics Technology Institute (KETI), Gwangju, Korea. E-mails: ohkhwan@keti.re.kr

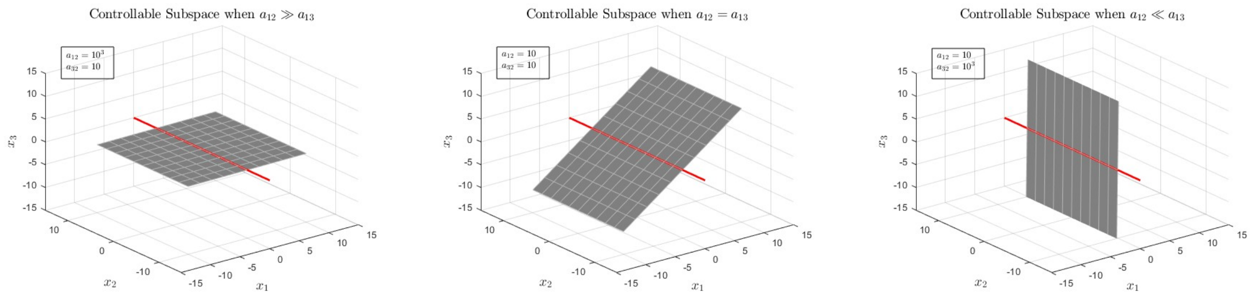


(a) $a_{12} \gg a_{32}$ (b) $a_{12} = a_{32}$ (c) $a_{12} \ll a_{32}$

Fig. 1. The SCS of (4) exists in infinite realizations. (a) The SCS nearly aligns with the $x_1x_2$-plane when $a_{12}$ is dominant over $a_{32}$. (b) It shows a particular configuration when $a_{12}$ is equal to $a_{32}$. (c) The SCS almost aligns with the $x_2x_3$-plane when $a_{32}$ is dominant over $a_{12}$.

*controllability matrix $\mathcal{C}$. This implies that each column of $\mathcal{C}$ corresponds to a basis of the SCS. Since the only non-zero value in the first column of (4) is the second element, it follows that $x_2$ is always controllable regardless of the network parameters. Conversely, the elements in the second column depend on each other, indicating that the states $x_1$ and $x_3$ are interdependent. It follows that $x_1$ and $x_3$ cannot be controlled simultaneously; thus, it is feasible to control either the state pair $\{x_1, x_2\}$ or $\{x_2, x_3\}$. Furthermore, countless realizations of SCS can exist depending on the relationship between network parameters $a_{12}$ and $a_{32}$. Fig.1 illustrates three characteristic realizations of these SCSs under different network parameters. Notably, these SCSs rotate around the $x_2$-axis, as depicted by the red line in Fig.1, implying that all SCSs include the $x_2$-axis. This indicates that the Fixed Structurally Controllable Subspace (FSCS), formed by the intersection of all realizations of SCS, is the $x_2$-axis, thus, $x_2$ remains a controllable state for all realizations of SCS. Thus, the concept of fixed controllable subspace effectively identifies the states that are consistently controllable for variations in the network parameters.*

In our technical note, the following propositions are key to determining *Fixed Structurally Controllable (FSC) nodes*.

**Proposition 1.** [1] For a graph $\mathcal{G}(\mathcal{V}, \mathcal{E})$, the dimension of SCS is the maximum number of state nodes that can be covered by a disjoint set of stems and cycles in $\mathcal{G}(\mathcal{V}, \mathcal{E})$.

Note that while the disjoint sets of stems and cycles within a graph may not be uniquely determined, the maximum number of state nodes contained in such a set remains unique.

**Proposition 2.** [2] For a graph $\mathcal{G}(\mathcal{V}, \mathcal{E})$, a state node $k \in \mathcal{V}$ is an FSC node if and only if $k$ becoming a leader with additional input does not increase the dimension of SCS.

Using **Proposition 1** and **Proposition 2**, the following example demonstrates how to determine FSC nodes.

**Example 3.** *Let us consider a graph $\mathcal{G}(\mathcal{V}, \mathcal{E})$ with a leader $1 \in \mathcal{V}_\mathcal{L}$ as shown in Fig. 2(c). A possible disjoint set of stems and cycles that covers the maximum number of state nodes includes the stem $(1 \rightarrow 2)$ and the cycle $(4 \rightarrow 5 \rightarrow 6 \rightarrow 4)$. From **Proposition 1**, the dimension of SCS for this configuration is 5. Now, if we consider state node 2 becoming a leader with additional input, i.e., $2 \in \mathcal{V}_\mathcal{L}$, the disjoint set could be reconfigured to include two stems: $(1 \rightarrow 3)$ and $(2 \rightarrow 4 \rightarrow 5 \rightarrow 6)$. In this case, the total number of state nodes covered by the two disjoint stems increases to 6, exceeding the original dimension of SCS. From **Proposition 2**, this outcome implies that state node $2 \in \mathcal{V}$ is not an FSC node. A similar increase in the dimension of SCS is observed if state node 3 becomes a leader. However, if state node 4, 5, or 6 becomes a leader, the dimension of SCS remains unchanged, thereby qualifying state nodes 4, 5, and 6 as FSC nodes. Note that adding multiple inputs to a state node, such as the leader $1 \in \mathcal{V}_\mathcal{L}$, does not affect the dimension of SCS, making these nodes trivially FSC nodes. Thus, the FSC nodes of the graph depicted in Fig. 2(c) are 1, 4, 5, and 6.*

The following example illustrates the necessity of the *Fixed Strongly Structurally Controllable Subspace (FSSCS)* concept, which we introduced in our technical note. It also highlights the differences between FSSCS and the *Fixed Structurally Controllable Subspace (FSCS)* concept proposed in [2].

**Example 4.** *Let us consider a graph $\mathcal{G}(\mathcal{V}, \mathcal{E})$ with a leader $1 \in \mathcal{V}_\mathcal{L}$ as shown in Fig. 2(d). Then, the corresponding structured*

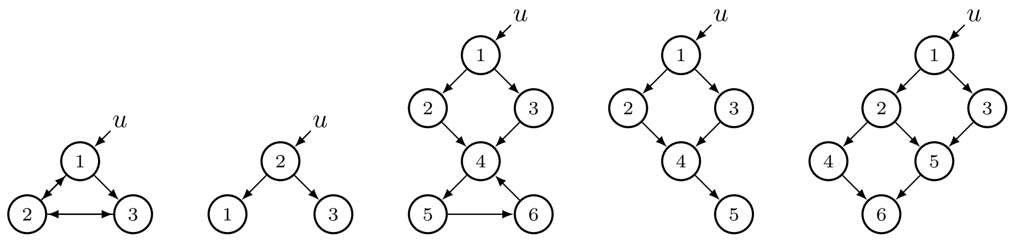

(a) $\mathcal{G}(\mathcal{V}, \mathcal{E})$ (b) $\mathcal{G}(\mathcal{V}, \mathcal{E})$ (c) $\mathcal{G}(\mathcal{V}, \mathcal{E})$ (d) $\mathcal{G}(\mathcal{V}, \mathcal{E})$ (e) $\mathcal{G}(\mathcal{V}, \mathcal{E})$

Fig. 2. Illustrative graphs for examples. (a) A graph that is structurally controllable but not strongly structurally controllable. (b) Example demonstrating the necessity of the fixed controllable subspace. (c) According to **Proposition 1**, the dimension of SCS is 5, with FSC nodes identified as $1, 4, 5$, and $6$. (d) Example highlighting the role of *multi-terms* in the controllability matrix. (f) Based on **Theorem 2**, in the controllability matrix of $\mathcal{G}(\mathcal{V}, \mathcal{E})$, either the *multi-term* in the 6-th row or the 5-th row cannot be zero.

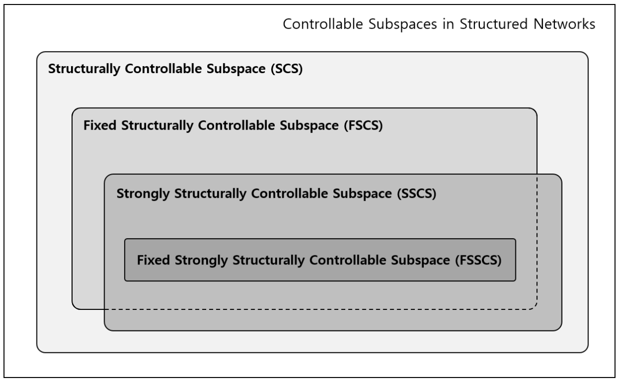


Fig. 3. Diagram illustrating the inclusion relationships among four types of controllable subspaces in a structured network.

*network is characterized by the following $\mathcal{A}_\mathcal{P}$ and $\mathcal{B}$:*

$$\mathcal{A}_\mathcal{P} = \begin{bmatrix} 0 & 0 & 0 & 0 & 0 \\ a_{21} & 0 & 0 & 0 & 0 \\ a_{31} & 0 & 0 & 0 & 0 \\ 0 & a_{42} & a_{43} & 0 & 0 \\ 0 & 0 & 0 & a_{54} & 0 \end{bmatrix}, \quad \mathcal{B} = \begin{bmatrix} 1 \\ 0 \\ 0 \\ 0 \\ 0 \end{bmatrix}. \tag{5}$$

*The controllability matrix for the pair $(\mathcal{A}_\mathcal{P}, \mathcal{B})$ is given by:*

$$\mathcal{C} = \begin{bmatrix} 1 & 0 & 0 & 0 & 0 \\ 0 & a_{21} & 0 & 0 & 0 \\ 0 & a_{31} & 0 & 0 & 0 \\ 0 & 0 & \alpha & 0 & 0 \\ 0 & 0 & 0 & a_{54}\alpha & 0 \end{bmatrix}, \tag{6}$$

*where $\alpha = a_{21}a_{42} + a_{31}a_{43}$. Each row vector in (6), denoted as $r_k \in \mathbb{R}^{1\times 5}$, corresponds to the state $x_k$ for $k \in \{1, \dots, 5\}$, clarifying the representation of each state in the controllability matrix. The controllability matrix in (6) has a rank of 4 when $\alpha \neq 0$ and a rank of 2 when $\alpha = 0$. Thus, the dimensions of the SCS and SSCS are 4 and 2, respectively. First, consider the case when $\alpha \neq 0$ to analyze the FSCS. In this case, $r_2$ and $r_3$ are dependent, while $r_1$, $r_4$, and $r_5$ are independent. As a result, states $x_2$ and $x_3$ cannot be controlled simultaneously, but states $x_1$, $x_4$, and $x_5$ maintain controllability under almost all network parameters. Therefore, $x_1$, $x_4$, and $x_5$ are included in the FSCS and remain controllable for all realizations of the SCS (i.e., they are controllable for almost all network parameters). Next, consider the case when $\alpha = 0$ to analyze the FSSCS. In this case, $r_4$ and $r_5$ become zero vectors. Since $r_2$ and $r_3$ remain dependent, only state $x_1$ is consistently controllable for all realizations of the SSCS (i.e., it is controllable for all network parameters). This example demonstrates that even though states $x_4$ and $x_5$ are included in the FSCS, they may become uncontrollable under specific realizations of network parameters, e.g., $\alpha = 0$. This shows a critical distinction in the robustness of controllability offered by the FSSCS compared to the FSCS. The inclusion relationships among the four types of controllable subspaces introduced in our technical note are shown in Fig. 3.*

The following example demonstrates the graph-theoretical meaning of the controllability matrix in a structured network, based on the concept of the *sum of weight products (SWP)* introduced in **Section IV** in our technical note.

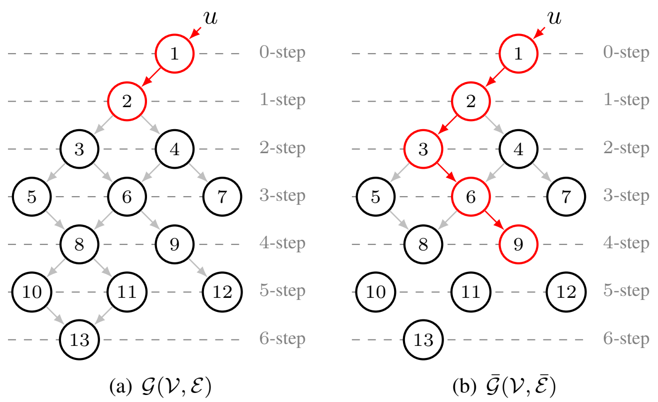


Fig. 4. Comparison between the dimensions of SSCS obtained using the derived set and subgraph approaches. (a) Result of the color-change rule. (c) Subgraph $\bar{\mathcal{G}}(\mathcal{V},\bar{\mathcal{E}})$ of $\mathcal{G}(\mathcal{V},\mathcal{E})$ obtained by **Algorithm 1**.

**Example 5.** *Let us consider the controllability matrix corresponding to the graph shown in Fig. 2(d) with a leader* $1 \in \mathcal{V}_{\mathcal{L}}$.

$$\mathcal{C} = \begin{bmatrix} 1 & 0 & 0 & 0 & 0 \\ 0 & a_{12} & 0 & 0 & 0 \\ 0 & a_{13} & 0 & 0 & 0 \\ 0 & 0 & \alpha & 0 & 0 \\ 0 & 0 & 0 & a_{45}\alpha & 0 \end{bmatrix}, \tag{7}$$

*where* $\alpha = a_{12}a_{24} + a_{13}a_{34}$. *Let us consider the stems from the leader to the state nodes in* $\mathcal{V}$ *with* $k$*-steps, where* $k \in \{0, \dots, 4\}$. *Then, each* $k$*-step from the leader corresponds to the* $(k+1)$*-th column vector in* $\mathcal{C}$. *Specifically, the* $i$*-th element in* $(k+1)$*-th column vector represents the SWP of all stems leading to the state node* $i \in \mathcal{V}$ *with* $k$*-steps. We now analyze the stems by sequentially increasing the steps from the leader. For the* ***0-step***, *the only node reachable from the leader is the leader itself, node* 1. *Thus,* $[\mathcal{C}]_{1,1}$ *holds the input connection weight of 1, indicating direct control by the external input. Moving to the* ***1-step***, *nodes* 2 *and* 3 *are reachable from the leader. Each of these nodes has a unique stem leading to it. Specifically, their SWPs are reflected as* $[\mathcal{C}]_{2,2} = a_{12}$ *and* $[\mathcal{C}]_{3,2} = a_{13}$, *respectively. At the* ***2-step***, *node* 4 *is reachable from the leader. This is achieved by two distinct stems:* $(1 \to 2 \to 4)$ *and* $(1 \to 3 \to 4)$, *the WPs of these stems are* $a_{12}a_{24}$ *and* $a_{13}a_{34}$, *respectively. Hence, the SWP for these stems is* $[\mathcal{C}]_{4,3} = a_{12}a_{24} + a_{13}a_{34}$, *illustrating the cumulative effect of the leader through multiple stems. For the* ***3-step***, *we observe that only node* 5 *is reachable. Similar to the previous step, there are two stems leading to node* 5*:* $(1 \to 2 \to 4 \to 5)$ *and* $(1 \to 3 \to 4 \to 5)$. *The SWP of these stems is* $[\mathcal{C}]_{5,4} = a_{45}(a_{12}a_{24} + a_{13}a_{34})$. *Lastly, at the* ***4-step***, *there are no reachable nodes from the leader, thus the fifth column of the controllability matrix being a zero vector.*

The following example illustrates a scenario where, despite the potential for *multi-terms* to become zero, dependencies on network parameters prevent all *multi-terms* in the controllability matrix from becoming zero.

**Example 6.** *Let us consider the following controllability matrix of the graph depicted in Fig. 2(e).*

$$\mathcal{C} = \begin{bmatrix} 1 & 0 & 0 & 0 & 0 & 0 \\ 0 & a_{12} & 0 & 0 & 0 & 0 \\ 0 & a_{13} & 0 & 0 & 0 & 0 \\ 0 & 0 & a_{12}a_{24} & 0 & 0 & 0 \\ 0 & 0 & \alpha & 0 & 0 & 0 \\ 0 & 0 & 0 & a_{56}\alpha + a_{12}a_{24}a_{46} & 0 & 0 \end{bmatrix}, \tag{8}$$

*where* $\alpha = a_{12}a_{25} + a_{13}a_{35}$. *The elements* $[\mathcal{C}]_{5,3}$ *and* $[\mathcal{C}]_{6,4}$ *are multi-terms, implying their potential to be zero. However, due to the dependency on network parameters, only one of these multi-terms can become zero. For instance, setting* $\alpha$ *to zero makes the element* $[\mathcal{C}]_{6,4}$ *a single-term, which is invariably non-zero. On the other hand, if* $a_{56}\alpha + a_{12}a_{24}a_{46}$ *is set to zero, we have* $\alpha = -a_{12}a_{24}a_{46}/a_{56}$, *which means the element in* $[\mathcal{C}]_{5,3}$ *cannot be zero.*

The following example demonstrates how to identify FSC and FSSC nodes using **Proposition 2** and **Theorem 1**, respectively.

**Example 7.** *Let us denote the sets of FSC and FSSC nodes as* $\mathcal{V}^{\text{FSC}}$ *and* $\mathcal{V}^{\text{FSSC}}$, *respectively. Consider the graph* $\mathcal{G}(\mathcal{V},\mathcal{E})$ *depicted in Fig 4. According to* ***Proposition 2***, *the FSC nodes in* $\mathcal{G}(\mathcal{V},\mathcal{E})$ *are identified as* $\mathcal{V}^{\text{FSC}} = \{1, 2, 13\}$. *These nodes are characterized by the property that their assumption as a leader does not lead to an increase in the dimension of SCS, which can be determined by* ***Proposition 1***. *Next, we analyze the FSSC nodes in* $\mathcal{G}(\mathcal{V},\mathcal{E})$. *According to* ***Theorem 1***, *the nodes that do not lead to an increase in the dimension of SSCS upon becoming a leader are classified as FSSC nodes. To determine*

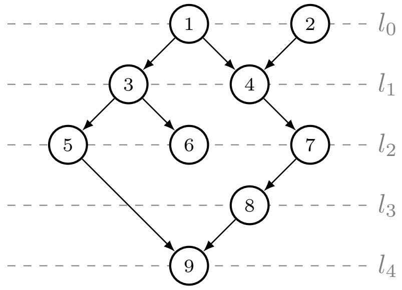


(a) DAG

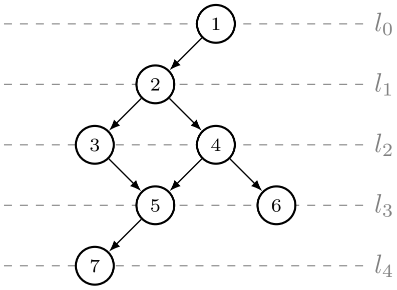


(b) HDAG

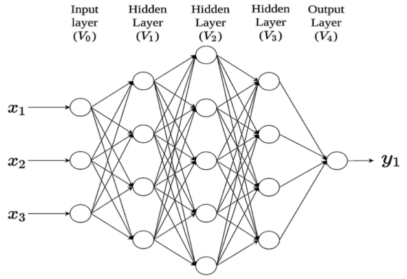


(c) Neural Network [3]

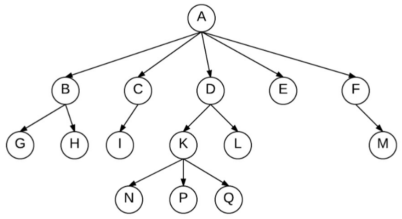


(d) Hierarchical organizations [4]

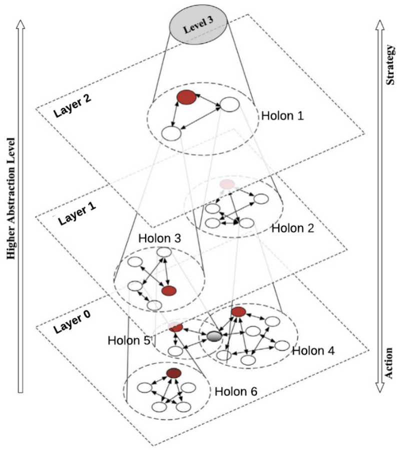


(e) Holonic organization [4]

Fig. 5. (a) In a DAG, edges between non-adjacent layers are allowed (e.g., $5 \to 9$ from $l_3$ to $l_5$). (b) In an HDAG, edges between non-adjacent layers are not allowed. (c) Basic structure of a neural network. (d) Hierarchical organizations as introduced in [4]. (e) Holonic organizations as introduced in [4].

*the dimension of SSCS, let us consider the subgraph $\bar{\mathcal{G}}(\mathcal{V}, \bar{\mathcal{E}})$ constructed by* ***Algorithm 1****. Specifically, in the graph depicted in Fig 4(b), the first step where only integrators or intermediators satisfying* ***Lemma 3*** *are reachable, occurs at the* 4*-steps. Hence, the subgraph $\bar{\mathcal{G}}(\mathcal{V}, \bar{\mathcal{E}})$ is defined by removing all edges connected to nodes reachable in and after* 4*-steps as illustrated in Fig 4(b). Utilizing this subgraph, we can apply* ***Theorem 4*** *to determine the dimension of SSCS for the original graph $\mathcal{G}(\mathcal{V}, \mathcal{E})$. From* ***Theorem 4*** *and* ***Theorem 1****, the nodes that do not increase the dimension of SSCS when becoming a leader are* 1 *and* 2*. Thus, the set of FSSC nodes is determined as $\mathcal{V}^{FSSC} = \{1, 2\}$.*

## II. Difference between DAG and HDAG

This section explains the intuitive differences between Hierarchical Directed Acyclic Graphs (HDAGs) and general Directed Acyclic Graphs (DAGs), as introduced in the technical note. According to [5], [6], every DAG can be represented as a hierarchical (or layered) structure. The algorithm introduced in [6] for partitioning an input-connected DAG into a unique hierarchical structure is as follows:

- **Initialization:** Remove all incoming edges of leaders.
- **Step 1:** Nodes without incoming edges are labeled as the top layer $l_0$, representing the highest level of influence.
- **Step 2:** Remove all nodes in layer $l_0$. Nodes in the remaining graph without incoming edges are labeled as layer $l_1$.
- **Step 3:** Repeat **Step 2** until all nodes are assigned a layer.

The initialization step ensures that any incoming edges to the leaders are removed, as leaders are directly controlled by external inputs, making such edges from other nodes redundant. Consequently, the top layer ($l_0$) consists solely of leaders. Every DAG can thus be uniquely partitioned into a hierarchical structure. This structure prohibits edges between nodes within the same layer and allows only directed edges from higher to lower layers. An important characteristic of DAGs is that **edges between non-adjacent layers are allowed**. For example, as shown in Fig. 5(a), a DAG can have edges like $5 \to 9$, which connect the non-adjacent layers $l_3$ and $l_5$. In the case of HDAGs, the only difference from DAGs is that **edges between non-adjacent layers are not allowed**. Edges in HDAGs are restricted to connecting only consecutive layers, i.e., from $l_k$ to $l_{k+1}$. This restriction ensures a top-down stream hierarchical structure between layers. Thus, while HDAGs retain most of the structural

properties of DAGs, they impose additional constraints. This constraint, as introduced in the technical note, requires that the sets $\mathcal{V}_k$ are mutually disjoint for $k \in \{1, \ldots, p\}$, where $\mathcal{V}_k$ represents the set of nodes reachable from the leader in exactly $k$-steps. In this sense, HDAGs are more generalized than tree structures but represent a more structured form of DAGs.

## III. Relation between FSSC Nodes and FSSCS

This section elaborates on the relationship between FSSC nodes and the FSSCS, as highlighted in **Remark 1** of the technical note. Specifically, **Theorem 1** in the technical note demonstrates that all standard basis vectors forming the FSSCS have a one-to-one correspondence with the FSSC nodes; that is, if a node is identified as an FSSC node, its corresponding standard basis vector is guaranteed to be in the FSSCS, and conversely, any standard basis vector in the FSSCS corresponds to an FSSC node. However, an arbitrary vector, other than the standard basis vectors, may serve as a basis for the FSSCS. For instance, consider a graph $\mathcal{G}(\mathcal{V}, \mathcal{E})$, where $\mathcal{V}^{\text{FSSC}} \subseteq \mathcal{V}$ denotes the set of FSSC nodes. According to **Theorem 1**, the basis of the FSSCS $\mathcal{C}_\Gamma^{\mathcal{F}}$ includes all the standard basis vectors corresponding to the FSSC nodes. Thus, if we define the space spanned by the standard basis vectors corresponding to the FSSC nodes as:

$$\mathcal{C}_\Gamma^{\text{FSSC}} = \text{span}\{v_i \in \mathbb{R}^n \mid i \in \mathcal{V}^{\text{FSSC}}\},$$

it holds that $\mathcal{C}_\Gamma^{\text{FSSC}} \subseteq \mathcal{C}_\Gamma^{\mathcal{F}}$. While all unit vectors (standard basis vectors) in the basis of $\mathcal{C}_\Gamma^{\mathcal{F}}$ have a one-to-one correspondence with the FSSC nodes, there could also be other non-unit vectors in the basis. Therefore, this does not imply that the FSSCS is uniquely determined by the standard basis vectors of the FSSC nodes.

Nonetheless, this result is sufficient to address the primary goal of the technical note, which is to identify the conditions for the independent strong structural controllability of individual nodes. For example, suppose that the FSSCS contains arbitrary vectors in its basis instead of standard basis vectors. This would mean that the FSSCS could take the form of a tilted two-dimensional plane in a three-dimensional space, as illustrated in Fig. 1(b). In such a case, $x_2$ would always be independently controllable, but $x_1$ and $x_3$ would exhibit dependency, making them not independently controllable. Since the technical note focuses on identifying FSSC nodes that ensure the independent strong structural controllability of individual nodes, it is sufficient to determine the unit vectors (or standard basis vectors) in the basis of the FSSCS.

## IV. Applications

This section introduces the applications of HDAGs and FSSC nodes as introduced in the technical note. These applications demonstrate their utility and significance across various domains, particularly in hierarchical networks and dynamic systems.

### A. Applications of HDAG

HDAG structures are frequently observed in neural networks as shown in Fig 5(c). For instance, neural networks have layered architectures similar to those of HDAGs, which served as an inspiration for this study. While these networks primarily focus on learning and representation, applying the controllability concepts explored in our technical note directly is challenging. However, HDAGs demonstrate greater practical relevance in the domain of Multi-Agent Systems (MAS), as highlighted in surveys like [4]. MAS applications span diverse fields, including security [7]–[9], learning [10], [11], fault detection [12], [13], localization [14]–[16], task allocation [17]–[19], controllability [20]–[22], and formation control [23]–[25].

Among the representative structures in MAS, systems with a hierarchical structure similar to HDAGs are often referred to as **Hierarchical Multi-Agent Systems (HMAS)**. The hierarchical structure of HMAS facilitates improved performance and efficiency in MAS by enhancing reliability, stability, flexibility, adaptability, and efficient resource utilization [26]. These benefits make HMAS a popular research area, as summarized in *Table I.* According to [4], the structure of HMAS can be broadly categorized into the following two types:

- **Hierarchical organizations:** As shown in Fig. 5(d), agents are arranged in a tree-like structure. Child agents communicate through parent agents, while parent agents control their children. At the top of the hierarchy, a root agent oversees all interactions, creating a centralized system.

- **Holonic organizations:** As shown in Fig. 5(e), agents are grouped into holons based on specific features, such as heterogeneity or sensing capabilities. Each holon forms a unit with a defined internal hierarchy, where the most resource-rich agents typically lead the group. Holons are then layered hierarchically, with higher-layer holons acting as super-agents that coordinate tasks collaboratively with lower-layer holons. This structure can be viewed as an extension of hierarchical organizations, where individual agents are replaced by holons, effectively representing groups of agents.

Hierarchical organizations can be considered centralized systems where all agents are controlled by a root agent, forming a tree structure. HDAGs provide a more general framework than this tree structure. In contrast, holonic organizations consist of

TABLE I
SUMMARY OF HIERARCHICAL MULTI-AGENT SYSTEMS (HMAS) REFERENCES

| Topic | Ref. | Contents |
|---|---|---|
| **Optimization and Resource Management** | [26] | HMAS-based multi-group structure for improving optimization performance |
| | [27] | HMAS design for traffic network signal optimization |
| | [28] | HMAS approach for resource allocation optimization in cloud computing |
| **Energy Systems and Microgrid Control** | [29] | HMAS-based energy coordination in islanded multi-microgrids |
| | [30] | HMAS implementation for black start operations in microgrids |
| | [31] | Hierarchical hybrid HMAS control for smart microgrids |
| **Dynamic System Stability and Resilience** | [32] | HMAS architecture for resilient dynamic control systems |
| | [33] | Achieving exponential consensus and stability in systems with hierarchical topology |
| | [34] | Hierarchical strategies for shape control and global convergence |
| **Learning-Based Systems and Behavioral Modeling** | [35] | Developing cooperative learning frameworks and algorithms in HMAS |
| | [36] | Behavioral modeling of HMAS with low-rank interactions |
| **General Frameworks and Applications** | [37] | General structures and algorithms for HMAS |
| | [38] | HMAS-based energy management and scheduling for electric vehicles |

groups (or clusters) that maintain hierarchical relationships. Although holonic organizations resemble hierarchical organizations in structure, they generalize individual agents into groups, where relationships between groups form a tree graph. Similar to HDAGs, holonic organizations only allow interactions between adjacent layers. However, within each layer, group interactions create dynamics distinct from HDAGs. Thus, holonic organizations cannot be classified as more general or restrictive than HDAGs but represent an alternative hierarchical structure. However, if condensation (or clustering) is applied to treat each group as a single node, holonic organizations can also be represented as a tree structure. Such cases, if each group is interpreted as a subsystem, the controllability of each subsystem can be analyzed using the theories proposed in the technical note.

If the tree structure of such HMAS is extended to an HDAG, it becomes possible to enable flexible inter-layer interactions while maintaining the hierarchical structure. For example, **HDAGs allow multiple parent agents to cooperatively control shared child agents, which is not feasible in traditional tree structures.** From the perspective of control in MAS, this flexibility provides significant advantages in applications such as:

- **Smart Grids:** In HDAG-based systems, multiple power sources (parents) can jointly manage a shared energy storage node (child), allowing flexible and cooperative energy distribution strategies. This enables more efficient balancing of supply and demand, which is not feasible in traditional tree-based hierarchies.
- **Distributed Sensor Networks:** HDAG structures allow two or more parent sensor clusters to relay complementary data to a shared aggregation node, enabling richer and more robust data integration compared to tree structures where each child node can only connect to a single parent.
- **Collaborative Robotics:** In HDAG configurations, two supervising robots (parents) can simultaneously coordinate the actions of a shared worker robot (child), improving the system's ability to handle complex tasks that require input or guidance from multiple sources.
- **Microgrid Control:** Multiple local energy controllers (parents) can cooperatively manage a single microgrid node (child) that oversees energy distribution across a specific area, ensuring greater flexibility and robustness in energy management compared to strictly hierarchical tree structures.
- **Traffic Signal Optimization:** Two upstream traffic controllers (parents) can jointly optimize the signal timing of a critical intersection (child), enabling more efficient traffic flow in complex urban networks where multiple roads converge.
- **Fleet Management for Autonomous Vehicles:** Two regional fleet managers (parents) can coordinate the operations of a shared set of autonomous vehicles (child), ensuring more adaptive and cooperative routing decisions that account for diverse regional constraints.

Thus, compared to traditional tree structures in HMAS, HDAGs maintain their hierarchical organization while enabling system designs and problem definitions that better reflect advanced real-world networks. Hence, the HDAG structure offers significant potential for practical applications in systems that require a hierarchical structure combined with the flexibility of inter-layer interactions.

### B. Applications of FSSC Nodes

FSSC nodes represent the most robust form of controllability in structured networks. By definition, FSSC nodes remain controllable for all possible realizations of network parameters, specifically, against variations in the values of non-zero patterns. From the perspective of control robustness, this makes them invaluable in dynamic and uncertain environments where network parameters may fluctuate due to external influences or internal adjustments. In structured networks, non-zero edge weights often represent dynamic properties such as communication strength, resource allocation, or signal transmission efficiency. These weights are subject to change due to environmental factors, system updates, or operational demands. In this case, FSSC nodes provide a guarantee of controllability that is invariant to such changes. This unique property enables their use as critical control points in systems that require reliable and consistent operation.

For instance, in multi-agent systems, FSSC nodes can serve as critical agents responsible for ensuring controllability within the structured network, even as interaction strengths (e.g., communication weights) between agents fluctuate. This property is particularly valuable in scenarios where local control and adaptability are crucial, such as robotic swarm coordination or autonomous vehicle platooning. In these contexts, while overall network performance may be influenced by varying weights, the roles assigned to FSSC nodes ensure that specific control tasks within their controllable subspace remain unaffected, enhancing local stability and reliability. Similarly, in energy distribution networks, FSSC nodes can be leveraged for key tasks such as load balancing or fault isolation. The robustness of FSSC nodes guarantees that these tasks can be carried out effectively regardless of variations in power flows or grid configurations. This property simplifies the design of adaptive control strategies, ensuring critical functions are consistently maintained even in dynamic environments. Beyond specific examples, FSSC nodes offer a valuable framework for analyzing and optimizing structured networks. By focusing on nodes that remain controllable under all parameter variations, system designers can allocate resources more effectively, develop simplified control strategies, and build networks resilient to uncertainties. This capability underscores the importance of FSSC nodes in advancing both theoretical research and practical applications in dynamic systems.

In conclusion, as elaborated in **Section IV-A**, the extensive applicability of HDAGs across a variety of domains highlights their potential to captivate a wide audience and make meaningful contributions to both academic research and practical implementations. Similarly, as emphasized in **Section IV-B**, FSSC nodes form the backbone of robust network design by ensuring controllability under all parameter variations. This capability makes them indispensable for reliably executing critical tasks across diverse applications. By leveraging the unique properties of FSSC nodes, researchers and practitioners can develop systems that are resilient, efficient, and adaptive.

## V. Comparison with Existing Results on the Lower Bounds of the Dimension of SSCS

Here we compare the dimension of SSCS obtained from existing results with that derived from the proposed **Theorem 4**. First, the work by [39] demonstrates that the maximum cardinality of the derived set serves as a lower bound for the dimension of SSCS. For simplicity, we explain this concept assuming a single leader in the network. The *color-change rules* used to determine the derived set are as follows:

- Initially, the leader in $\mathcal{V}_{\mathcal{L}}$ are colored red, and the other state nodes are colored black.
- If a red node has only one black out-neighbor node, then the black node is colored red.

For a graph $\mathcal{G}(\mathcal{V}, \mathcal{E})$, the set of red nodes that emerges when the *color-change rule* becomes inapplicable is called the derived set, denoted as $\mathcal{D}(\mathcal{G})$. Then, let us consider the following proposition that provides a lower bound for the dimension of SSCS.

**Proposition 3.** [39] For a graph $\mathcal{G}(\mathcal{V}, \mathcal{E})$ with a leader, the dimension of SSCS is lower bounded by the cardinality of the derived set in $\mathcal{G}(\mathcal{V}, \mathcal{E})$.

The following example shows the difference between the results obtained from **Proposition 3** and **Theorem 4**.

**Example 8.** *Let us consider the HDAG $\mathcal{G}(\mathcal{V}, \mathcal{E})$ shown in Fig. 4(a). First, applying the color-change rules to the graph, node $2$ is forced by the leader, node $1$. After that, since node $2$ has two white out-neighbor nodes $3, 4 \in \mathcal{V}$, the color-change rules cannot be further applied. Ultimately, we obtain the derived set as $\mathcal{D}(\mathcal{G}) = \{1, 2\}$ as shown in Fig. 4(b). Consequently, the lower bound on the dimension of SSCS obtained by **Proposition 3** is 2, i.e., $|\mathcal{D}(\mathcal{G})| = 2$. On the other hand, let us consider the subgraph $\bar{\mathcal{G}}(\mathcal{V}, \bar{\mathcal{E}})$ obtained by **Algorithm 1** as shown in Fig. 4(c). From **Theorem 4**, we obtain the exact dimension of SSCS as 5, which is larger than the dimension of SSCS obtained by **Proposition 3**.*

# VI. Complexity Analysis

In this section, we analyze the computational complexity of **Proposition 2**, which provides the necessary and sufficient condition for determining FSC nodes, and **Theorem 1**, which provides the necessary and sufficient condition for determining FSSC nodes as presented in our technical note.

## A. *Complexity of* ***Proposition 2***

First, we examine the complexity of **Proposition 2**. For a graph $\mathcal{G}(\mathcal{V},\mathcal{E})$, the complexity of determining FSC nodes under **Proposition 2** is based on identifying whether a state node in $\mathcal{V}$ increases the dimension of the SCS when it becomes an additional leader. **Proposition 1** provides the condition for determining the dimension of SCS, which is equivalent to the number of nodes consisting of disjoint stems and cycles included in the maximum matching [40]. This maximum matching can be efficiently computed using the Hopcroft–Karp algorithm, with a complexity of $O(|\mathcal{E}|\sqrt{|\mathcal{V}|})$ [41]. When this process is applied to each state node in $\mathcal{V}$, the overall complexity for determining FSC nodes becomes $O(|\mathcal{V}||\mathcal{E}|\sqrt{|\mathcal{V}|})$, which remains polynomial. Note that while maximum matching finds disjoint paths and cycles, if the search is initiated by the leaders, it can identify disjoint stems and cycles. Specifically, by starting the search from the leaders, the number of nodes in the disjoint stems and cycles obtained from the maximum matching corresponds to the dimension of SCS.

## B. *Complexity of* ***Theorem 1***

Next, the necessary and sufficient condition for determining FSSC nodes is provided as follows:

**Theorem 1.** For a graph $\mathcal{G}(\mathcal{V},\mathcal{E})$, a state node $i \in \mathcal{V}$ is an FSSC node if and only if $i$ becoming a leader with additional input does not increase the dimension of SSCS.

To determine FSSC nodes, the exact dimension of SSCS is required. To achieve this, the subgraph $\bar{\mathcal{G}}(\mathcal{V},\bar{\mathcal{E}})$ of the given graph $\mathcal{G}$ must first be constructed, as detailed in **Algorithm 1**. The condition and lemma for this process are as follows:

**Condition 1.** For an integrator $i_w \in \mathcal{V}^{int}$ in $\mathcal{G}(\mathcal{V},\mathcal{E})$, there exists exactly one stem leading to $i_w$ that does not include any other integrator. By the definition of integrators, this condition ensures the existence of at least one additional stem leading to $i_w$ that includes another integrator $i_l \in \mathcal{V}^{int}$, where $i_w \neq i_l$.

**Lemma 4.** For a graph $\mathcal{G}(\mathcal{V},\mathcal{E})$ with an integrator $i_w \in \mathcal{V}^{int}$ satisfying **Condition 1**, consider a column $c_k$ in the controllability matrix that consists only of *multi-terms* including the *multi-term* of $i_w$. All the *multi-terms* in column $c_k$ can become zero if and only if there is no intermediator among the nodes corresponding to these *multi-terms* that passes through the integrator $i_l$ from the leader.

To analyze the complexity of obtaining the subgraph $\bar{\mathcal{G}}(\mathcal{V},\bar{\mathcal{E}})$ using **Algorithm 1**, we will break down the process into the following three stages:

- **Stage 1:** Complexity to find integrators $i_w$ and $i_l$ in **Condition 1**.
- **Stage 2:** Complexity to find columns that consists only of *multi-terms* including the *multi-term* of $i_w$ in **Lemma 4**.
- **Stage 3:** Complexity to find the intermediator that passes through the integrator $i_l$ from the leader in **Lemma 4**.

**Stage 1.** In a general *directed acyclic graph* (DAG) with a single leader, finding an integrator $i_w$ that satisfies **Condition 1** would require finding all paths from the leader to each node, which could have exponential complexity of $\mathcal{O}(2^{|\mathcal{V}|})$. However, since we are dealing with *hierarchical directed acyclic graphs* (HDAGs), all paths from the leader to each node become the shortest paths. Therefore, we can use Dijkstra's Algorithm with polynomial complexity of $\mathcal{O}(|\mathcal{E}|\log|\mathcal{V}|)$. Although the standard Dijkstra algorithm typically returns only a single shortest path even if multiple paths with the same length exist, we can modify the algorithm to keep track of all such paths in the priority queue without increasing the time complexity. (This modification may increase the space complexity, it remains polynomial.) Thus, the overall complexity for finding an integrator $i_w$ that satisfies **Condition 1** across all nodes will be $\mathcal{O}(|\mathcal{V}| \times |\mathcal{E}|\log|\mathcal{V}|)$. If no integrator $i_w$ satisfies **Condition 1**, a breadth-first search (BFS) with complexity $\mathcal{O}(|\mathcal{V}|+|\mathcal{E}|)$ can be used to find the first $k$-step where all nodes are integrators or intermediators, enabling us to easily construct the subgraph for the dimension of SSCS using **Algorithm 1**. If an integrator $i_w$ satisfying **Condition 1** is found, we then move on to **Stages 2 and 3** to check **Lemma 4**.

**Stage 2.** Finding a column consisting only of *multi-terms* including the *multi-term* of $i_w$ in **Lemma 4** is equivalent to finding the $k$-steps where nodes reachable from the leader are either integrators or intermediators. This can also be done using BFS with a complexity of $\mathcal{O}(|\mathcal{V}|+|\mathcal{E}|)$.

**Stage 3.** If an integrator $i_w$ satisfying **Condition 1** is found in **Stage 1**, then another integrator $i_l$ can also be identified. The problem of finding the intermediator that passes through the integrator $i_l$ from the leader is equivalent to finding the shortest paths from $i_l$ to nodes with one incoming edge (intermediators). As the step increases and no intermediator satisfies **Lemma 4**, this step, $k_{first}$, is determined. In **Algorithm 1**, all edges connected to nodes reachable beyond $k_{first}$ are removed, resulting in the subgraph $\bar{\mathcal{G}}(\mathcal{V}, \bar{\mathcal{E}})$. Hence, the final complexity to construct a subgraph under **Algorithm 1** remains at most $\mathcal{O}(|\mathcal{V}| \times |\mathcal{E}| \log |\mathcal{V}|)$.

With this subgraph, the complexity of verifying whether the dimension of SSCS increases when a node becomes a leader with additional input is equivalent to that of **Proposition 1**, which is $\mathcal{O}(|\mathcal{E}|\sqrt{|\mathcal{V}|})$. Applying this verification to every node results in an overall complexity of $\mathcal{O}(|\mathcal{V}||\mathcal{E}|\sqrt{|\mathcal{V}|})$ for determining all FSSC nodes in an HDAG using **Theorem 1**.

**Algorithm 1** Constructing Subgraph Corresponding to $\bar{C}$

**Input:** A graph $\mathcal{G}(\mathcal{V}, \mathcal{E})$ with $|\mathcal{V}| = n$
Initialize $\mathcal{E}' = \emptyset$
**for** $k = 1$ **to** $n - 1$ **do**
  $\mathcal{V}_k \leftarrow$ nodes reachable from the leader with $k$-steps
  **if** $\mathcal{V}_k$ consists only of integrators or intermediators, with no intermediators satisfying **Lemma 4 then**
    $k_{first} \leftarrow k$
    **break**
  **end if**
**end for**
**for** $k = k_{first}$ **to** $n - 1$ **do**
  $\mathcal{V}_k \leftarrow$ nodes reachable from the leader with $k$-steps
  $\mathcal{E}_k \leftarrow$ edges connected with nodes in $\mathcal{V}_k$
  $\mathcal{E}' \leftarrow \mathcal{E}' \cup \mathcal{E}_k$
**end for**
$\bar{\mathcal{E}} \leftarrow \mathcal{E} \setminus \mathcal{E}'$
**Output:** Subgraph $\bar{\mathcal{G}}(\mathcal{V}, \bar{\mathcal{E}})$

## References


[1] S. Hosoe. Determination of generic dimensions of controllable subspaces and its application. *IEEE Transactions on Automatic Control*, 25(6):1192–1196, 1980.

[2] C. Commault, J. Van Der Woude, and T. Boukhobza. On the fixed controllable subspace in linear structured systems. *Systems & Control Letters*, 102:42–47, 2017.

[3] O. A. Montesinos-López, A. Montesinos-López, and J. Crossa. *Fundamentals of artificial neural networks and deep learning*, pages 379–425. Springer, 2022.

[4] A. Dorri, S. S. Kanhere, and R. Jurdak. Multi-agent systems: A survey. *IEEE Access*, 6:28573–28593, 2018.

[5] Y.-Y. Liu, J.-J. Slotine, and A.-L. Barabási. Control centrality and hierarchical structure in complex networks. *PLoS ONE*, 7(9):e44459, 2012.

[6] N.-J. Park, Y.-U. Kim, and H.-S. Ahn. Fixed node determination and analysis in directed acyclic graphs of structured networks. *Journal of the Franklin Institute*, page 106995, 2024.

[7] H. Yu, Z. Shen, C. Leung, C. Miao, and V. R. Lesser. A survey of multi-agent trust management systems. *IEEE Access*, 1:35–50, 2013.

[8] X. Wang, M. Maghami, and G. Sukthankar. Leveraging network properties for trust evaluation in multi-agent systems. In *2011 IEEE/WIC/ACM International Conferences on Web Intelligence and Intelligent Agent Technology*, volume 2, pages 288–295. IEEE, 2011.

[9] R. C. Cavalcante, I. I. Bittencourt, A. P. da Silva, M. Silva, E. Costa, and R. Santos. A survey of security in multi-agent systems. *Expert Systems with Applications*, 39(5):4835–4846, 2012.

[10] K.-S. Hwang, W.-C. Jiang, and Y.-J. Chen. Model learning and knowledge sharing for a multiagent system with dyna-q learning. *IEEE Transactions on Cybernetics*, 45(5):978–990, 2014.

[11] D. Chakraborty and P. Stone. Multiagent learning in the presence of memory-bounded agents. *Autonomous Agents and Multi-Agent Systems*, 28:182–213, 2014.

[12] M. R. Davoodi, K. Khorasani, H. A. Talebi, and H. R. Momeni. Distributed fault detection and isolation filter design for a network of heterogeneous multiagent systems. *IEEE Transactions on Control Systems Technology*, 22(3):1061–1069, 2013.

[13] J. R. Koza. *Genetic Programming II: Automatic Discovery of Reusable Programs*. MIT Press, 1994.

[14] M. Saim, K. Munawar, and U. Al-Saggaf. An overview of localization methods for multi-agent systems. *International Journal of Engineering Research and Applications*, 7(01):19–24, 2017.

[15] S. Jafari, A. Ajorlou, and A. G. Aghdam. Leader localization in multi-agent systems subject to failure: A graph-theoretic approach. *Automatica*, 47(8):1744–1750, 2011.

[16] S. Bandini, S. Manzoni, and G. Vizzari. Multi-agent approach to localization problems: The case of multilayered multi-agent situated system. *Web Intelligence and Agent Systems: An International Journal*, 2(3):155–166, 2004.

[17] S. S. Fatima and M. Wooldridge. Adaptive task resources allocation in multi-agent systems. In *Proceedings of the Fifth International Conference on Autonomous Agents*, pages 537–544, 2001.

[18] F. Rahimzadeh, L. M. Khanli, and F. Mahan. High reliable and efficient task allocation in networked multi-agent systems. *Autonomous Agents and Multi-Agent Systems*, 29:1023–1040, 2015.

[19] V. Singhal and D. Dahiya. Distributed task allocation in dynamic multi-agent system. In *International Conference on Computing, Communication & Automation*, pages 643–648. IEEE, 2015.

[20] L. Wang, F. C. Jiang, G. M. Xie, and Z. Ji. Controllability of multi-agent systems based on agreement protocols. *Science in China Series F: Information Sciences*, 52(11):2074–2088, 2009.

[21] A. Rahmani, M. Ji, M. Mesbahi, and M. Egerstedt. Controllability of multi-agent systems from a graph-theoretic perspective. *SIAM Journal on Control and Optimization*, 48(1):162–186, 2009.

[22] M. Zamani and H. Lin. Structural controllability of multi-agent systems. In *2009 American Control Conference*, pages 5743–5748. IEEE, 2009.

[23] X. Ge and Q.-L. Han. Distributed formation control of networked multi-agent systems using a dynamic event-triggered communication mechanism. *IEEE Transactions on Industrial Electronics*, 64(10):8118–8127, 2017.

[24] F. Xiao, L. Wang, J. Chen, and Y. Gao. Finite-time formation control for multi-agent systems. *Automatica*, 45(11):2605–2611, 2009.

[25] D. Li, S. S. Ge, W. He, G. Ma, and L. Xie. Multilayer formation control of multi-agent systems. *Automatica*, 109:108558, 2019.

[26] M. Roshanzamir, M. A. Balafar, and S. N. Razavi. A new hierarchical multi group particle swarm optimization with different task allocations inspired by holonic multi agent systems. *Expert Systems with Applications*, 149:113292, 2020.

[27] M. K. Tan, H. S. E. Chuo, R. K. Y. Chin, K. B. Yeo, and K. T. K. Teo. Hierarchical multi-agent system in traffic network signalization with improved genetic algorithm. In *2018 IEEE International Conference on Artificial Intelligence in Engineering and Technology (IICAIET)*, pages 1–6. IEEE, 2018.

[28] X. Gao, R. Liu, and A. Kaushik. Hierarchical multi-agent optimization for resource allocation in cloud computing. *IEEE Transactions on Parallel and Distributed Systems*, 32(3):692–707, 2020.

[29] M. Ding, K. Ma, R. Bi, M. Mao, and L. Chang. A hierarchical control scheme based on multi-agent system for islanded multi-microgrids. In *2013 4th IEEE International Symposium on Power Electronics for Distributed Generation Systems (PEDG)*, pages 1–5. IEEE, 2013.

[30] N. Cai, X. Xu, and J. Mitra. A hierarchical multi-agent control scheme for a black start-capable microgrid. In *2011 IEEE Power and Energy Society General Meeting*, pages 1–7. IEEE, 2011.

[31] C.-X. Dou and B. Liu. Multi-agent based hierarchical hybrid control for smart microgrid. *IEEE Transactions on Smart Grid*, 4(2):771–778, 2013.

[32] C. Rieger and Q. Zhu. A hierarchical multi-agent dynamical system architecture for resilient control systems. In *2013 6th International Symposium on Resilient Control Systems (ISRCS)*, pages 6–12. IEEE, 2013.

[33] Z. Duan, G. Zhai, and Z. Xiang. Exponential consensus for hierarchical multi-agent systems with switching topology and inter-layer communication delay. *IET Control Theory & Applications*, 10(4):451–460, 2016.

[34] T. Sugie, F. Tong, B. D. O. Anderson, and Z. Sun. On global convergence of area-constrained formations of hierarchical multi-agent systems. In *2020 59th IEEE Conference on Decision and Control (CDC)*, pages 2805–2810. IEEE, 2020.

[35] M. Ghavamzadeh, S. Mahadevan, and R. Makar. Hierarchical multi-agent reinforcement learning. *Autonomous Agents and Multi-Agent Systems*, 13:197–229, 2006.

[36] H. Shimizu and S. Hara. Cyclic pursuit behavior for hierarchical multi-agent systems with low-rank interconnection. In *2008 SICE Annual Conference*, pages 3131–3136. IEEE, 2008.

[37] A. Wakulicz-Deja and M. Przybyła-Kasperek. *Hierarchical multi-agent system*. Recent Advances in Intelligent Information Systems, Academic Publishing House EXIT, 2009.

[38] C. B. Saner, A. Trivedi, and D. Srinivasan. A cooperative hierarchical multi-agent system for ev charging scheduling in presence of multiple charging stations. *IEEE Transactions on Smart Grid*, 13(3):2218–2233, 2022.

[39] A. Y. Yazicioglu, M. Shabbir, W. Abbas, and X. Koutsoukos. Strong structural controllability of diffusively coupled networks: Comparison of bounds based on distances and zero forcing. In *Proc. IEEE 59th Conference on Decision and Control*, pages 566–571, 2020.

[40] J. Gao, Y.-Y. Liu, R. M. D'souza, and A.-L. Barabási. Target control of complex networks. *Nature Communications*, 5(1):1–8, 2014.

[41] J. E. Hopcroft and R. M. Karp. An nˆ5/2 algorithm for maximum matchings in bipartite graphs. *SIAM Journal on Computing*, 2(4):225–231, 1973.
